# Supplementary material for: Sparse Probability of Agreement
Source: arXiv:2208.06161 source file (2023-02-24)
Supplement: Supplementary file 1 [file chance_correction_bound.tex]

\section{Bias of Chance Correction}

\inote{
	Use
	\begin{itemize}
		\item \url{https://www.stat.cmu.edu/~hseltman/files/ratio.pdf}
		\item \url{http://markirwin.net/stat110/Lecture/Section74.pdf}
		\item \url{https://statmd.wordpress.com/2013/08/04/the-expectation-of-the-ratio-of-two-random-variables/}
	\end{itemize}
}

Fleiss kappa is computed by
\begin{align}
	\kappa = 1 - \frac{1 - \bar{P}}{1 - \bar{P}_e},
\end{align}
where 
\begin{align}
	 \bar{P}_o &= \frac{1}{\sum_i n_i (n_i - 1)} \sum_i \sum_c n_{ic} (n_{ic} - 1) \nonumber \\
	 \bar{P}_e &= \sum_c \left( \frac{\sum_i n_{ic}}{\sum_i n_i} \right)^2 \nonumber \\
	 	&= \frac{1}{\l(\sum_i n_i\r)^2} \sum_c \left( \sum_i n_{ic} \right)^2
\end{align}

We now randomly change the number $n_{i'c'}$. The variance of these two components are
\begin{align}
	\var[\bar{P}_o] &= \frac{1}{\sum_i n_i (n_i - 1)} \var[ n_{i'c'} (n_{i'c'} - 1) ] \nonumber \\ 
	\var[\bar{P}_e] &= \frac{1}{\l(\sum_i n_i\r)^2} \var\l[ n_{i'c'}^2 + 2 n_{i'c'} \sum_c n_{i'c} \r]  \nonumber
\end{align}

We note that
\begin{align}
	\var[ n_{i'c'} (n_{i'c'} - 1) ] \leq \var\l[ n_{i'c'}^2 \r] \\
	 \leq \var\l[ n_{i'c'}^2 + 2 n_{i'c'} \sum_c n_{i'c} \r], \nonumber
\end{align}

but what about the fraction? \\

we would like to have
\begin{align}
	\var[\bar{P}_o] \leq \var[\bar{P}_e].
\end{align}
